# Supplementary material for: Found in the Middle: Permutation Self-Consistency Improves Listwise Ranking in Large Language Models
Source: arXiv:2310.07712 source file (2024-04-22)
Supplement: Supplementary file 1 [file appendix.tex]

% Suppose we sample an input ranking uniformly from $\mathcal{S}_{|X|}$, i.e., $\boldsymbol{R}^\text{in} \sim \textsc{Unif}(\mathcal{S}_{|X|})$. % because prior, we can't take list order for granted
% Then, define the \textit{output ranking} random variable (r.v.) as
% \begin{equation}
%     \boldsymbol{R}^\text{out} := h(X[\boldsymbol{R}^\text{in}_i]; s).\label{eqn:llm-sample}
% \end{equation}
% As previously remarked~\cite{citeme}, this output represents a nonconstant distribution because the LLM's outputs change for different $\boldsymbol{R}^\text{in}$ (e.g., positional bias). % noisy, not being a constant, What is this in other words
% Our distribution of interest is then $\Pr(\boldsymbol{R}^\text{out}|\boldsymbol{\sigma}_y)$ since ....
% We parameterize this using the Mallows ranking model with the Kendall tau distance, which is popular in the machine learning literature~\cite{citeme}:
% \begin{equation}
%     \Pr(\bs{R}^\text{out} | \bs{\sigma}_y) := \frac{e^{-d_\kappa(\bs{\sigma}_y, \bs{R}^\text{out})}}{\sum_{\bs{\sigma}'\in\mathcal{S}_{|X|}} e^{-d_\kappa(\bs{\sigma}_y, \bs{\sigma}')}}.
% \end{equation} % write intuition here, such as sigma y centers
% The output of permutation self-consistency then is the optimal $\bs{\sigma}_y^*$ that maximizes the likelihood of this model, i.e., % high-level effect of this?
% \begin{equation}
%     \bs{\sigma}_y^* := \argmax_{\bs\sigma} \Pr(\bs{r}^\text{out}_1, \dots, \bs{r}^\text{out}_N |\bs\sigma_y=\bs\sigma)
% \end{equation}\\[-5ex]
% \begin{equation}\small
%     = \argmax_{\bs\sigma} \Pr(\bs{r}^\text{out}_1 |\bs\sigma_y=\bs\sigma) \cdots \Pr(\bs{r}^\text{out}_N |\bs\sigma_y=\bs\sigma),
% \end{equation}
% for realizations $\bs{r}^\text{out}_1, \dots, \bs{r}^\text{out}_N$ of $\bs{R}^\text{out}$, drawn by passing a sample of the input list ranking r.v. $\bs{R}^\text{in}$  through the LLM (Eqn.~\ref{eqn:llm-sample}). % resulting from passing ... plain english
% % We call this sample of output rankings an \textit{output batch} for short.






% \section{Our Approach}

% \subsection{Preliminaries}
% \parheader{Notation}
% We define a \textit{ranking} as a vector $\bs r \in \{1, \dots, n\}^n$, where $\bs r_i \neq \bs r_j$ for any $i \neq j$.
% For some $n$-element set $S$, define $S[\bs r]$ as the permutation of $S$ under the total order induced by $\bs r$, where $S[\boldsymbol r]_i$ precedes $S[\boldsymbol r]_j$ if $\boldsymbol r_i < \boldsymbol r_j$.
% To quantify dissimilarity, let the Kendall tau distance between two rankings be the number of pairwise disagreements, or \textit{discordant} pairs:
% \begin{gather*}\scriptstyle
%     d_{\kappa}\left(\bs r^{(1)}, \bs r^{(2)}\right) := \sum_{\substack{1 \leq i < j \leq n}} \mathbb{I}((\boldsymbol r^{(1)}_i < \boldsymbol r^{(1)}_j \wedge \boldsymbol r^{(2)}_i > \boldsymbol r^{(2)}_j) \vee\\\scriptstyle\hspace{39.5mm} (\boldsymbol r^{(1)}_i > \boldsymbol r^{(1)}_j \wedge \boldsymbol r^{(2)}_i < \boldsymbol r^{(2)}_j)),
% \end{gather*}
% where $\mathbb{I}$ is the indicator function.
% The distance is one affine transform away from the Kendall tau correlation, used to measure list order similarity~\cite{citeme}:
% \begin{equation}
% \tau(\boldsymbol r^{(1)}, \boldsymbol r^{(2)}) := 1 - \frac{2d_{\kappa}(\boldsymbol r^{(1)}, \boldsymbol r^{(2)})}{\binom{n}{2}}.
% \end{equation}
% In the extreme, $\tau=1 \iff \bs{r}^{(1)} = \bs r^{(2)}$, and $\tau=-1$ implies that one is the other's reverse.

% \subsection{Permutation Self-Consistency}
% How do we mitigate positional biases in listwise-ranking LLMs?
% We find inspiration in the self-consistency framework~\cite{citeme}, which improves both quality and consistency in chain-of-thought prompting~\cite{citeme}.
% The approach has two main stages: first, it \textit{samples} multiple answers for an input prompt; then, it \textit{aggregates} the sampled answers into a single, high-quality one, hence ``marginalizing out'' separate reasoning paths from the LLM.

% Self-consistency unfortunately does not readily generalize to listwise ranking for a few reasons.
% For one, it is limited to point predictions, greatly simplifying the aggregation procedure to taking the majority vote.
% For another, sampling temperature, the method's mainstay of generating diverse samples for aggregation, has little effect on (and at times harming) the quality of aggregated predictions in listwise ranking, as shown in Section~\red{X}.
% Lastly, self-consistency does not explicitly address positional bias, the central issue of our paper.

% Nevertheless, its sample--aggregate paradigm serves as a useful template for us.
% For the first sampling step, we randomly shuffle the list in the prompt to curate a diverse set of rankings, each with different position biases.
% For the next aggregation step, we compute the central ranking closest in Kendall tau distance to all the sampled rankings.
% Intuitively, we intervene on list order, collect output rankings, then produce an aggregate ranking, breaking the association between individual list order and predictions.

% Formally, we are given an input set of items $X$, such as a list of passages, along with a listwise-ranking LLM $h(X; s)$ that returns a ranking of length $|X|$ on some string prompt $s$; see Figure~\red{X} for an example.
% First, we construct a diverse set of output rankings by randomly permuting $X$ and passing it through the LLM, like how self-consistency uses temperature to vary their output.
% Specifically, we sample a sequence
% \begin{equation}
%     \hat{\bs r}^{(i)} := h(X[\bs\pi^{(i)}]; s)\text{ for }1 \leq i \leq m,
% \end{equation}
% where $\bs\pi^{(i)}$ are rankings drawn randomly from the set of all possible rankings of length $|X|$.
% As noted previously, each output ranking has positional bias, but mistakes are expected to differ among the outputs because of our input order randomization.
% We then ``marginalize out'' these individual biases by aggregating the output rankings into a single central ranking.
% One method with attractive theoretical properties is the Kemeny--Young~\cite{citeme} optimal ranking of the outputs---that is, the central ranking that minimizes the sum of its Kendall tau distances to every output ranking:
% \begin{equation}
%     \bar{\bs r} := \argmin_{\bs r^*}\sum_{1 \leq i \leq m} d_\kappa(\hat{\bs r}^{(i)}, \bs r^*).
% \end{equation}
% Our permutation self-consistency algorithm returns $\bar{\bs r}$ as the prediction for $X$ and concludes.
% Although this calculation is NP-hard, efficient exact algorithms~\cite{citeme} and fast approximations exist~\cite{citeme}, many implemented in our codebase.

% \parheader{Passage reranking}
% Ranking a set of provided documents in order of relevance to a query is the task of passage reranking.
% The specific use of permutation self-consistency for this deserves special attention, as predominant LLMs such as RankGPT~\cite{citeme} and RankVicuna~\cite{citeme} do not output rankings in a single inference pass, since the document context can exceed the maximum length.
% Instead, they reorder fixed windows of items from the back of the list to the front, calling the LLM for each stride; see Figure~\red{X}.
% In this case, we simply apply permutation self-consistency to each window call.

% \parheader{Theoretical guarantees}
% We now show that for certain kinds of noisy rankings, the Kemeny--Young ranking can recover the true ranking given enough observations.
% For example, if there always exists some random pair of items that are correctly ranked among randomly ordered observations, we will converge to the true ranking.

% \begin{definition}
%     For two rankings $\bs r$ and $\bs r'$, the concordant subset is a set $S'$ where $\forall i$ and $ j \in S', \bs r_i < \bs r_j \wedge \bs r'_i < \bs r'_j$ or $\bs r_i > \bs r_j \wedge \bs r'_i > \bs r'_j$. % what is ordering pair?
% \end{definition}
